# Supplementary material for: Ultrafast Energy Transfer with Competing Channels: Non-equilibrium Foerster and Modified Redfield Theories
Source: arXiv:1701.08684 ancillary file (2017-01-30)
Supplement: Supplementary file 1 [file supporting_info.pdf]

# Ultrafast Energy Transfer with Competing Channels: Non-equilibrium Förster and Modified Redfield Theories, Supporting Information

Joachim Seibt and Tomáš Mančal*
*Faculty of Mathematics and Physics, Ke Karlovu 5, 121 16 Prague 2, Czech Republic*

### Derivation of non-equilibrium Modified Redfield transfer rates

By applying a generating function approach [1] with parameters $a$ and $a'$, the Modified Redfield transfer rate for non-equilibrated bath in the initial exciton state $k$ can be formulated as

$$\begin{aligned}\mathcal{R}_{kkk'k',bath}(a,a',t) = 2\Re\left(\int_0^t dt' Tr_q\left\{\exp(iH^0_{k'}t)\exp\left(ia\sum_n a_{k'k}(n)u_n\right)\exp(-iH^0_k t)\right.\right.\\ \left.\left.\exp(iH^0_k t')\exp\left(-ia'\sum_n a_{kk'}u_n\right)\exp(-iH^0_{k'}t')\rho_{b,eq,g}\right\}\right).\end{aligned} \tag{1}$$

The derivation of the rate expression in terms of line shape functions consists of the following steps: First, the transformation of the energy gap coordinate to the interaction picture via

$$u_k(\tau) = \exp(ie^{ph}_k\tau)u_k\exp(-ie^{ph}_k\tau). \tag{2}$$

leads to the appearance of time-ordered exponentials [2] in the expression

$$\begin{aligned}\mathcal{R}_{kkk'k',bath}(a,a',t) &= 2\Re\left(\int_0^t dt'\exp(i(E^0_{k'}-E^0_k)(t-t'))\right.\\ &\prod_n Tr_q\left\{\exp(i(a^2_{k'k'}(n)l_n - a^2_{kk}(n)l_n)(t-t'))\right.\\ &\exp_-\left[i\int_0^t d\tau a_{k'k'}(n)u_n(\tau)\right]\exp(ie^{ph}_n t)\exp(iaa_{k'k}(n)u_n)\exp(-ie^{ph}_n t)\\ &\exp_+\left[-i\int_0^t d\tau a_{kk}(n)u_n(\tau)\right]\exp_-\left[i\int_0^{t'} d\tau a_{kk}(n)u_n(\tau)\right]\\ &\exp(ie^{ph}_n t')\exp(-ia'a_{kk'}(n)u_n)\exp(-ie^{ph}_n t')\\ &\left.\left.\exp_+\left[-i\int_0^{t'} d\tau a_{k'k'}(n)u_n(\tau)\right]\exp(-be^{ph}_n)\right\}\right)\\ &= 2\Re\left(\int_0^t dt'\exp(i(E^0_{k'}-E^0_k)t')\prod_n r^{(n)}_{kkk'k',bath}(t,t',a,a')\right).\end{aligned} \tag{3}$$

Then the transfer rate can be obtained via

$$\begin{aligned}\mathcal{R}_{kkk'k',bath}(t) &= \lim_{a,a'\to 0}\frac{\partial^2}{\partial a\partial a'}(\mathcal{R}_{kkk'k',bath}(a,a',t))\\ &= 2\Re\left(\int_0^t dt'\exp(i(E^0_{k'}-E^0_k)(t-t'))\lim_{a,a'\to 0}\frac{\partial^2}{\partial a\partial a'}\prod_n r^{(n)}_{kkk'k',bath}(t,t',a,a')\right).\end{aligned} \tag{4}$$

---

* tomas.mancal@mff.cuni.cz

with

$$
\begin{aligned}
&\lim_{a,a'\to 0}\frac{\partial^2}{\partial a\partial a'}\prod_n r^{(n)}_{kkk'k',bath}(t,t',a,a')\\
&=\prod_n Tr_q\left\{\exp(i(a^2_{k'k'}(n)-a^2_{kk}(n))l_n(t-t'))\exp_-\left[i\int_0^t d\tau a_{k'k'}(n)u_n(\tau)\right]\right.\\
&\exp(ie^{ph}_n t)\exp(iaa_{k'k}(n)u_n)\exp(-ie^{ph}_n t)\exp_+\left[-i\int_0^t d\tau a_{kk}(n)u_n(\tau)\right]\\
&\exp_-\left[i\int_0^{t'} d\tau a_{kk}(n)u_n(\tau)\right]\exp(ie^{ph}_n t')\exp(-ia'a_{kk'}(n)u_n)\exp(-ie^{ph}_n t')\\
&\left.\exp_+\left[-i\int_0^{t'} d\tau a_{k'k'}(n)u_n(\tau)\right]\exp(-be^{ph}_n)\right\}.
\end{aligned}
\tag{5}
$$

The generating functions can be expressed for infinitesimal $a$ and $a'$ as

$$
\begin{aligned}
&\exp(ie^{ph}_n t)\exp(iaa_{k'k}(n)u_n)\exp(-ie^{ph}_n t)=\exp\left[ia_{k'k}(n)u_n(t)a\right]=\exp\left[i\int_0^a d\tau a_{k'k}(n)u_n(t+\tau)\right]\\
&=\exp\left[i\int_0^{t+a} d\tau' a_{k'k}(n)u_n(\tau')\right]\exp\left[-i\int_0^{t} d\tau' a_{k'k}(n)u_n(\tau')\right]
\end{aligned}
\tag{6}
$$

and

$$
\begin{aligned}
&\exp(ie^{ph}_n t')\exp(-ia'a_{kk'}(n)u_n)\exp(-ie^{ph}_n t')=\exp\left[-ia_{kk'}(n)u_n(t')a'\right]\\
&=\exp\left[-i\int_0^{a'} d\tau a_{kk'}(n)u_n(t'+\tau)\right]\\
&=\exp\left[-i\int_0^{t'+a'} d\tau' a_{kk'}(n)u_n(\tau')\right]\exp\left[i\int_0^{t'} d\tau' a_{kk'}(n)u_n(\tau')\right],
\end{aligned}
\tag{7}
$$

where the exponentials are not time-ordered. By inserting Eqs. (6) and (7) into Eq. (5), one obtains

$$
\begin{aligned}
&\lim_{a,a'\to 0}\frac{\partial^2}{\partial a\partial a'}\prod_n r^{(n)}_{kkk'k',bath}(t,t',a,a')\\
&=\prod_n Tr_q\left\{\exp(i(a^2_{k'k'}(n)-a^2_{kk}(n))l_n(t-t'))\exp_-\left[i\int_0^t d\tau a_{k'k'}(n)u_n(\tau)\right]\right.\\
&\exp\left[i\int_0^{t+a} d\tau' a_{k'k}(n)u_n(\tau')\right]\exp\left[-i\int_0^{t} d\tau' a_{k'k}(n)u_n(\tau')\right]\exp_+\left[-i\int_0^t d\tau a_{kk}(n)u_n(\tau)\right]\\
&\exp_-\left[i\int_0^{t'} d\tau a_{kk}(n)u_n(\tau)\right]\exp\left[-i\int_0^{t'+a'} d\tau' a_{kk'}(n)u_n(\tau')\right]\exp\left[i\int_0^{t'} d\tau' a_{kk'}(n)u_n(\tau')\right]\\
&\left.\exp_+\left[-i\int_0^{t'} d\tau a_{k'k'}(n)u_n(\tau)\right]\exp(-be^{ph}_n)\right\}.
\end{aligned}
\tag{8}
$$

Second-order cumulant expansion of single time-ordered exponentials results in line shape functions

$$
g(\tau_1)=\int_0^{\tau_1} d\tau\int_0^{\tau} d\tau' Tr_q\left\{u_n(\tau)u_n(\tau')\right\},
\tag{9}
$$

whereas combinations of different first-oder expansion terms lead to expressions

$$
h(\tau_1,\tau_2)=\int_0^{\tau_1} d\tau\int_0^{\tau_2} d\tau' Tr_q\left\{u_n(\tau)u_n(\tau')\right\}=g(\tau_1)-g(\tau_1-\tau_2)+g(-\tau_2),
\tag{10}
$$

with $g(-\tau) = g^*(\tau)$, which appear independent of whether the expanded exponentials are time-ordered or not. Separate evaluation of the time-ordered exponentials results in exponentials with line shape function arguments

$$\begin{aligned} f_1(t,t') &= -g^*_{n,k'k'k'k'}(t) - g_{n,kkkk}(t) - g^*_{n,kkkk}(t') - g_{n,k'k'k'k'}(t') + h_{n,k'k'kk}(t,t) - h_{n,k'k'kk}(t,t') \\ &\quad + h_{n,k'k'k'k'}(t,t') + h_{n,kkkk}(t,t') - h_{n,kkk'k'}(t,t') + h_{n,kkk'k'}(t',t') \\ &= -g_{n,kkkk}(t-t') + g_{n,kkk'k'}(t-t') + g_{n,k'k'kk}(t-t') - g_{n,k'k'k'k'}(t-t') \\ &\quad + 2i\Im(g_{n,k'k'k'k'}(t)) - 2i\Im(g_{n,kkk'k'}(t)) - 2i\Im(g_{n,k'k'k'k'}(t')) + 2i\Im(g_{n,kkk'k'}(t')). \end{aligned} \tag{11}$$

The cumulant expansion terms with involvement of the terms resulting from Eqs. (6) and (7) are

$$\begin{aligned} f_2(t,t',a,a') = &-h_{n,k'k'k'k}(t,t+a) + h_{n,kkk'k}(t+a,t) - h_{n,kkk'k}(t+a,t') \\ &+ h_{n,k'kkk'}(t+a,t'+a') - h_{n,k'kkk'}(t+a,t') + h_{n,k'k'k'k}(t+a,t') \\ &+ h_{n,k'k'k'k}(t,t) - h_{n,kkk'k}(t,t) + h_{n,kkk'k}(t,t') \\ &- h_{n,k'kkk'}(t,t'+a') + h_{n,k'kkk'}(t,t') - h_{n,k'k'k'k}(t,t') \\ &+ h_{n,k'k'kk'}(t,t'+a') - h_{n,kkkk'}(t,t'+a') + h_{n,kkkk'}(t',t'+a') - h_{n,k'k'k'k}(t'+a,t') \\ &- h_{n,k'k'kk'}(t,t') + h_{n,kkkk'}(t,t') - h_{n,kkkk'}(t',t') + h_{n,k'k'k'k}(t',t'). \end{aligned} \tag{12}$$

Note that this expression vanishes in the limit of $a$ and $a'$ approaching zero, so the appearance of $f_2(t,t',a,a')$ as the argument of an exponential leads to a factor of 1. The derivatives with respect to $a$ and $a'$ in the limit of these parameters approaching zero lead to the expressions

$$\lim_{a\to 0}\frac{\partial}{\partial a} f_2(t,t',a,a') = -(\dot g_{n,k'kk'k'}(t-t') - \dot g_{n,k'kkk}(t-t') - 2i\Im(\dot g_{n,k'kk'k'}(t))) \tag{13}$$

and

$$\lim_{a'\to 0}\frac{\partial}{\partial a'} f_2(t,t',a,a') = \dot g_{n,k'k'kk'}(t-t') - \dot g_{n,kkkk'}(t-t') - 2i\Im(\dot g_{n,k'k'kk'}(t')). \tag{14}$$

Taking the mixed derivative results in a factor

$$\lim_{a,a'\to 0}\frac{\partial^2}{\partial a\partial a'} f_2(t,t',a,a') = \ddot g_{n,k'kkk'}(t-t') + \lim_{a\to 0}\frac{\partial}{\partial a} f_2(t,t',a,a') \lim_{a'\to 0}\frac{\partial}{\partial a'} f_2(t,t',a,a'). \tag{15}$$

Altogether the rate expression

$$\begin{aligned} \mathcal{R}_{kkk'k',bath}(t) = 2\Re\Bigg( \int_0^t & dt' \exp(i(E^0_{k'} - E^0_k)(t-t'))\exp(i(l_{k'k'k'k'} - l_{kkkk})(t-t')) \\ & \exp\left(-g_{kkkk}(t-t') + g_{kkk'k'}(t-t') + g_{k'k'kk}(t-t') - g_{k'k'k'k'}(t-t')\right. \\ & \left.+2i\Im(g_{k'k'k'k'}(t)) - 2i\Im(g_{kkk'k'}(t)) - 2i\Im(g_{k'k'k'k'}(t')) + 2i\Im(g_{kkk'k'}(t'))\right) \\ & \times \{\ddot g_{k'kkk'}(t-t') \\ & - [(\dot g_{k'kk'k'}(t-t') - \dot g_{k'kkk}(t-t') - 2i\Im(\dot g_{k'kk'k'}(t))))] \\ & \times [(\dot g_{k'k'kk'}(t-t') - \dot g_{kkkk'}(t-t') - 2i\Im(\dot g_{k'k'kk'}(t')))]\} \Bigg), \end{aligned} \tag{16}$$

is obtained. An analogous derivation of the inhomogeneous term leads to

$$\begin{aligned} \mathcal{I}_{kkk'k',bath}(t) = 2\Im & \left(\exp(-i(E^0_{k'} - E^0_k)t)\exp(-i(l_{k'k'k'k'} - l_{kkkk})t)\right. \\ & \exp(-g^*_{kkkk}(t) - g_{k'k'k'k'}(t) + g_{kkk'k'}(t) + g^*_{kkk'k'}(t)) \\ & \left.\times (\dot g^*_{k'kkk}(t) - \dot g_{k'kk'k'}(t))\right). \end{aligned} \tag{17}$$

---


[1] M. Yang and G. R. Fleming, Chemical Physics **275**, 355 (2002).
[2] S. Mukamel, *Principles of Nonlinear Spectroscopy* (Oxford University Press, Oxford, 1995).
